# Supplementary material for: Filling-enforced Dirac loops and their evolutions under various perturbations
Source: arXiv:2001.07107 source file (2020-01-20)
Supplement: Supplementary file 1 [file Supplementary_Materials.pdf]

| FEDL materials in SG.62 | Material Project ID | Symmetry indicator Z4 |
|---|---|---|
| Fe4 P4 | mp-1005 | 2 |
| Cs4 | mp-1007976 | 1 |
| Lu4 Pt4 | mp-1025438 | 3 |
| Y4 Pt4 | mp-1025448 | 3 |
| Sr4 Nb4 O12 | mp-10339 | 0 |
| Nb4 Si4 Pt4 | mp-10469 | 3 |
| Yb4 Si4 Ir4 | mp-10569 | 2 |
| Pr4 Pt4 | mp-1078557 | 1 |
| Lu4 Ni4 | mp-1078899 | 1 |
| Ho4 Pt4 | mp-1079180 | 1 |
| Tb4 Pt4 | mp-1079305 | 1 |
| Ba4 Al4 | mp-1079984 | 2 |
| Tb4 Pd4 | mp-1080451 | 1 |
| Yb4 Au4 | mp-1084808 | 1 |
| Ho4 Pd4 | mp-1087502 | 1 |
| Sc4 Ge4 Pt4 | mp-1095253 | 1 |
| Yb4 Ga4 Ni4 | mp-1095431 | 3 |
| Zr4 Ge4 Ir4 | mp-1095472 | 3 |
| Pb4 Cl4 O4 | mp-1095473 | 1 |
| La4 Sn4 Pd4 | mp-1095476 | 2 |
| Tm4 Si4 Pt4 | mp-1095501 | 0 |
| Hf4 Cu4 Ge4 | mp-1095504 | 0 |
| Sr4 Cd4 Au4 | mp-1095513 | 2 |
| Y4 Zn4 Pd4 | mp-1095522 | 0 |
| V4 Si4 Ni4 | mp-1095532 | 1 |
| Ta4 P4 Rh4 | mp-1095548 | 3 |
| Ta4 Co4 P4 | mp-1095553 | 3 |
| Tb4 Al4 Au4 | mp-1095572 | 2 |
| Y4 Ge4 Pt4 | mp-1095607 | 0 |
| Y4 Sn4 Pd4 | mp-1095628 | 2 |
| Tb8 Au4 | mp-1095658 | 2 |
| Sr4 In4 Pd4 | mp-1095684 | 2 |
| Tm8 Au4 | mp-1095690 | 2 |
| La4 Al4 Au4 | mp-1101778 | 2 |
| Lu8 Au4 | mp-1101816 | 2 |
| Nd8 Al4 | mp-1101848 | 1 |
| Zr4 Cu4 Sn4 | mp-1101867 | 3 |
| Ti4 Fe4 P4 | mp-1101870 | 3 |
| Lu4 Si4 Pt4 | mp-1101919 | 0 |
| Tl4 Pd8 | mp-1101944 | 3 |
| Nb4 P4 Rh4 | mp-1101948 | 3 |
| Zr4 Ge4 Rh4 | mp-1101959 | 3 |
| Nb4 Co4 As4 | mp-1101967 | 1 |
| Pr4 Al4 Au4 | mp-1101978 | 2 |
| V4 Co4 P4 | mp-1101982 | 3 |
| Nb4 Ni4 Ge4 | mp-1101995 | 3 |
| Hf4 Ni4 P4 | mp-1102032 | 0 |
| Ti4 Cu4 Ge4 | mp-1102042 | 3 |
| Sc4 Si4 Pd4 | mp-1102080 | 2 |
| Ti4 Ni4 As4 | mp-1102086 | 1 |
| Ga8 Au4 | mp-1102090 | 1 |
| Nd8 Au4 | mp-1102098 | 2 |
| Tm4 Ge4 Pt4 | mp-1102110 | 1 |
| Yb4 Al4 Pt4 | mp-1102117 | 3 |
| Tm4 Ni4 Sn4 | mp-1102179 | 0 |
| Ti4 Ni4 P4 | mp-1102188 | 3 |
| Pb4 I4 O4 | mp-1102199 | 1 |

| | | |
|---|---|---|
| Pb4 Br4 O4 | mp-1102225 | 2 |
| Yb4 Ga4 Pd4 | mp-1102228 | 3 |
| Tm4 Al4 Au4 | mp-1102248 | 2 |
| Pr4 Mg4 Sn4 | mp-1102281 | 3 |
| Yb8 Ga4 | mp-1102309 | 1 |
| Sm8 Al4 | mp-1102344 | 0 |
| As4 Rh8 | mp-1102364 | 2 |
| Ba8 In4 | mp-1102396 | 1 |
| Re4 N8 | mp-1102441 | 2 |
| Y4 Ga4 Rh4 | mp-1102458 | 3 |
| Sc4 Si4 Ru4 | mp-1102525 | 1 |
| Nb4 V4 P4 | mp-1102537 | 2 |
| Zr4 Co4 Si4 | mp-1102565 | 1 |
| Yb4 As4 S4 | mp-1102611 | 2 |
| Ca4 Al4 Pt4 | mp-1102631 | 0 |
| Nb4 Si4 Ni4 | mp-1102658 | 3 |
| Dy8 Al4 | mp-1102728 | 0 |
| La4 Zn4 Pd4 | mp-1102763 | 2 |
| Y4 Al4 Au4 | mp-1102840 | 2 |
| Hf4 Ge4 Ir4 | mp-1102841 | 1 |
| Fe4 Mo4 P4 | mp-1102843 | 0 |
| Zr4 Si4 Ir4 | mp-1102869 | 1 |
| Er8 Al4 | mp-1102875 | 0 |
| Ho4 Si4 Pt4 | mp-1102935 | 0 |
| Hf4 Ge4 Rh4 | mp-1102945 | 1 |
| Er8 Au4 | mp-1102972 | 2 |
| Zr4 P4 Os4 | mp-1102976 | 3 |
| Ho4 Al4 Au4 | mp-1102992 | 2 |
| Tm4 Zn4 Pd4 | mp-1103059 | 0 |
| Ho4 Ge4 Pt4 | mp-1103105 | 0 |
| Pr4 Ni4 Ge4 | mp-1103115 | 2 |
| Zr4 Cu4 Ge4 | mp-1103123 | 1 |
| Zr4 Co4 Ge4 | mp-1103148 | 3 |
| Ti4 Ge4 Ir4 | mp-1103158 | 1 |
| Y4 Si4 Pt4 | mp-1103176 | 2 |
| Ta4 Fe4 Ge4 | mp-1103196 | 3 |
| Ta4 Rh8 | mp-1103212 | 2 |
| Pr8 Al4 | mp-1103225 | 0 |
| Hf4 Co4 Si4 | mp-1103227 | 1 |
| Ti4 Si4 Ir4 | mp-1103248 | 3 |
| Y4 Ga4 Ir4 | mp-1103280 | 2 |
| Nb4 Ge4 Pt4 | mp-1103346 | 1 |
| Tb8 Al4 | mp-1103391 | 0 |
| La8 Au4 | mp-1103395 | 2 |
| Dy8 Au4 | mp-1103411 | 2 |
| Pr4 Ga4 Co4 | mp-1103498 | 1 |
| Ho4 Ga4 Co4 | mp-1103576 | 0 |
| Sm8 Au4 | mp-1103633 | 2 |
| Y4 Ni4 Ge4 | mp-1103655 | 0 |
| Tm8 Re4 C8 | mp-1105554 | 1 |
| Lu4 Si4 Pt8 | mp-1105597 | 2 |
| Y12 Ni4 | mp-1105633 | 2 |
| Ho4 Si4 Pd8 | mp-1105686 | 2 |
| Pr12 Ru4 | mp-1105741 | 0 |
| Yb12 Co4 | mp-1105958 | 3 |
| Pr4 Ge4 Pd8 | mp-1105974 | 3 |
| Ca4 B8 H4 | mp-1106103 | 3 |
| Pr12 Ni4 | mp-1106122 | 3 |

| | | |
|---|---|---|
| Y4 B8 Os4 | mp-1106229 | 3 |
| Yb4 Mg4 Au4 | mp-11080 | 2 |
| Yb4 Cd4 Au4 | mp-11085 | 2 |
| Lu4 In4 Rh4 | mp-11101 | 0 |
| Y8 Al4 | mp-11230 | 0 |
| Mg8 Au4 | mp-11250 | 0 |
| Si4 Ir4 | mp-1128 | 2 |
| Tm4 Ni4 | mp-11525 | 1 |
| Ho4 Sn4 Pd4 | mp-11764 | 2 |
| Yb4 Cu4 Pb4 Se12 | mp-1178694 | 1 |
| Tm4 W4 C8 | mp-1178946 | 0 |
| Ho4 B8 Ru4 | mp-1181033 | 3 |
| Ho4 W4 C8 | mp-1181041 | 0 |
| Ba4 Ag4 | mp-11840 | 1 |
| Ho8 Re4 C8 | mp-1184737 | 1 |
| Ir4 C12 | mp-1184780 | 0 |
| Ho4 Ni4 | mp-11871 | 1 |
| Ho4 Mo4 C8 | mp-1188132 | 0 |
| Dy8 Re4 C8 | mp-1188135 | 1 |
| Y4 Si4 Pt8 | mp-1188158 | 2 |
| Y4 B8 Ru4 | mp-1188195 | 3 |
| Lu8 Re4 C8 | mp-1188244 | 1 |
| Tm4 B8 Os4 | mp-1188249 | 3 |
| Tm4 Si4 Pd8 | mp-1188299 | 2 |
| Ho12 Pt4 | mp-1188476 | 3 |
| Tb4 Mo4 C8 | mp-1188505 | 0 |
| Tb4 B8 Ru4 | mp-1188601 | 3 |
| Tm4 B8 Ru4 | mp-1188615 | 3 |
| Y12 Os4 | mp-1188757 | 3 |
| Ta4 Ni4 P8 | mp-1188762 | 2 |
| Nb8 N12 | mp-1188869 | 3 |
| Pr4 Zn12 | mp-1188870 | 1 |
| Sc12 As8 | mp-1188926 | 2 |
| Tb4 Zn12 | mp-1188983 | 1 |
| Pr4 Si4 Pd8 | mp-1189045 | 2 |
| Lu4 Ge4 Pd8 | mp-1189057 | 2 |
| Sc4 B8 Os4 | mp-1189073 | 3 |
| Ho4 Ge4 Pd8 | mp-1189077 | 3 |
| Tm4 Ge4 Pd8 | mp-1189166 | 2 |
| Lu4 B8 Os4 | mp-1189270 | 3 |
| Tm12 Pt4 | mp-1189442 | 2 |
| Tb4 B8 Os4 | mp-1189495 | 3 |
| La12 Ni4 | mp-1189497 | 3 |
| Tb12 Os4 | mp-1189565 | 0 |
| Y4 W4 C8 | mp-1189574 | 0 |
| La12 Ru4 | mp-1189592 | 0 |
| Lu12 Pt4 | mp-1189834 | 2 |
| Ho4 B8 Os4 | mp-1189925 | 3 |
| Lu4 Si4 Pd8 | mp-1189950 | 2 |
| Y4 Mo4 C8 | mp-1189984 | 0 |
| Lu4 Zn12 | mp-1190019 | 1 |
| Tm4 Mo4 C8 | mp-1190031 | 0 |
| Ho4 Si4 Pt8 | mp-1190095 | 2 |
| Tb4 W4 C8 | mp-1190096 | 0 |
| Sr4 Al8 Au12 | mp-1190136 | 2 |
| Tm4 Si4 Pt8 | mp-1190240 | 2 |
| Ca4 B8 H12 | mp-1190960 | 0 |
| Sr4 B4 Pd16 | mp-1191090 | 1 |

| | | |
|---|---|---|
| Ba4 B4 Pd16 | mp-1191182 | 1 |
| Tm4 Ge8 Rh16 | mp-1192459 | 3 |
| Y4 Ge8 Rh16 | mp-1192507 | 3 |
| La4 Sn16 Rh8 | mp-1193123 | 3 |
| Na4 Ru8 O16 | mp-1193175 | 0 |
| K4 Hg24 | mp-1193208 | 2 |
| Sc12 Si12 Ru4 | mp-1193608 | 2 |
| Pr4 Sn16 Rh8 | mp-1194179 | 3 |
| Sc12 Si12 Pt4 | mp-1194390 | 0 |
| Li4 Yb4 Ge8 | mp-11944 | 0 |
| Cd4 Cu4 As4 H4 O20 | mp-1195165 | 0 |
| Zr12 Sb28 Pd4 | mp-1195256 | 1 |
| Hf12 Ni4 Sb28 | mp-1195404 | 1 |
| Hf12 Sb28 Pd4 | mp-1195520 | 1 |
| Sr8 Al20 Pd16 | mp-1195613 | 1 |
| Li4 Ho16 Ge16 | mp-1195831 | 1 |
| Ho20 Ge16 | mp-1196008 | 1 |
| Ho4 Ni20 Ge12 | mp-1196011 | 2 |
| Ag4 Au4 F28 | mp-1196161 | 1 |
| Tm20 Ge16 | mp-1196455 | 0 |
| Li4 Nd16 Ge16 | mp-1196908 | 1 |
| Bi4 C8 O20 | mp-1197076 | 3 |
| Li4 Pr16 Ge16 | mp-1197150 | 1 |
| Tm12 Ni12 Sn24 | mp-1197522 | 1 |
| Y8 Nb12 Ge16 | mp-1197535 | 0 |
| La20 Rh16 | mp-1197877 | 0 |
| Nd8 Sb16 Ir12 | mp-1197956 | 2 |
| Ba4 Ge8 Au20 | mp-1198185 | 0 |
| La8 Sb16 Ir12 | mp-1198252 | 2 |
| Tb12 Ni12 Sn24 | mp-1198844 | 1 |
| Tb20 Pt16 | mp-1198980 | 0 |
| Ho20 Pt16 | mp-1198999 | 0 |
| Ni20 P20 | mp-1199085 | 1 |
| Lu20 Ge16 | mp-1199467 | 0 |
| Pr28 Si20 Ni8 | mp-1199517 | 3 |
| Lu24 Te8 Au4 | mp-1199600 | 2 |
| Cu24 Bi4 Se24 | mp-1199896 | 2 |
| Ca12 Ag12 Ge12 | mp-1200102 | 0 |
| Ho4 Si12 Ni20 | mp-1200132 | 2 |
| Hf8 Ni12 P12 | mp-1200507 | 2 |
| Ho20 Sb8 Pd4 | mp-1200650 | 0 |
| Sc8 Nb12 Si16 | mp-1200765 | 0 |
| Sc8 Nb12 Ge16 | mp-1200971 | 0 |
| Lu20 Pt16 | mp-1202267 | 2 |
| La28 Ru12 | mp-1202486 | 2 |
| Ho8 Nb12 Ge16 | mp-1202575 | 0 |
| Pr8 Sb16 Ir12 | mp-1202719 | 2 |
| Er8 Nb12 Ge16 | mp-1202972 | 0 |
| Hf8 Ni12 As12 | mp-1203331 | 2 |
| Ta32 Co4 Se32 | mp-1204251 | 2 |
| Dy8 Nb12 Ge16 | mp-1204364 | 0 |
| Y4 Ge4 Pd8 | mp-1207627 | 2 |
| Y12 Ru4 | mp-1207781 | 3 |
| Tm12 Ru4 | mp-1207837 | 3 |
| Tb4 Si4 Pd8 | mp-1208310 | 2 |
| Tb4 Ge4 Pd8 | mp-1208316 | 2 |
| Tb4 Si4 Pt8 | mp-1208318 | 2 |
| Tb12 Pt4 | mp-1208453 | 2 |

| | | |
|---|---|---|
| Y20 Pt16 | mp-12175 | 3 |
| La4 Ni4 Sn4 | mp-12613 | 2 |
| Ca8 Cu4 | mp-12614 | 3 |
| P4 Ru4 | mp-12636 | 2 |
| Ho4 Si4 | mp-12900 | 0 |
| Yb4 Zn4 Au4 | mp-13027 | 3 |
| Sr4 Li4 Ge8 | mp-13139 | 1 |
| Ba4 Li4 Ge8 | mp-13140 | 1 |
| Y20 Ge16 | mp-13360 | 1 |
| Th4 Cu20 Sn4 | mp-13413 | 0 |
| Hf4 Si4 Rh4 | mp-13472 | 1 |
| Lu4 Ge4 Pt4 | mp-13580 | 1 |
| Y4 Ni4 | mp-1364 | 3 |
| Li4 Ca4 Si8 | mp-13916 | 2 |
| Li4 Ca4 Ge8 | mp-13917 | 2 |
| As4 Ru4 | mp-15650 | 2 |
| Si16 Ir12 | mp-15656 | 2 |
| Re8 P4 | mp-1637 | 2 |
| La4 Pd4 O12 | mp-16415 | 0 |
| Ho8 Al4 | mp-16502 | 0 |
| Al4 Pt8 | mp-16526 | 2 |
| Tb20 Ge16 | mp-1673 | 0 |
| Yb20 Sb12 | mp-16826 | 3 |
| Hf20 Sb12 | mp-17466 | 1 |
| Mg4 Ni8 P4 | mp-17942 | 2 |
| Li4 Cu8 O8 | mp-18162 | 1 |
| La4 Si4 | mp-1860 | 0 |
| V4 S4 | mp-1868 | 2 |
| Ga4 Pd8 | mp-1869 | 0 |
| Pr20 Ge16 | mp-1908 | 0 |
| Tb4 Si4 | mp-1924 | 0 |
| Yb4 Cu4 | mp-1937 | 1 |
| U4 Si4 Ir4 | mp-19806 | 1 |
| P4 Pd12 | mp-19879 | 2 |
| Yb4 Cu4 S8 | mp-19888 | 0 |
| Lu4 Ni4 Ge4 | mp-19922 | 0 |
| Ce4 Ge4 Ir4 | mp-20022 | 3 |
| U4 Si4 Rh4 | mp-20184 | 1 |
| Pr4 Ru4 O12 | mp-20186 | 0 |
| Hf4 Mn4 Si4 | mp-20192 | 1 |
| U4 Ge4 Ir4 | mp-20226 | 0 |
| Mn4 Co4 P4 | mp-20249 | 3 |
| Ti4 Cu4 Si4 | mp-20255 | 0 |
| Tm4 Si4 Ru4 | mp-20308 | 3 |
| U4 Ge4 Rh4 | mp-20321 | 0 |
| Mn4 Nb4 P4 | mp-20335 | 0 |
| Sr4 Pr4 O12 | mp-20464 | 0 |
| Yb4 Ge4 Rh4 | mp-20498 | 2 |
| B4 Pd12 | mp-20517 | 1 |
| Cu4 S4 O16 | mp-20525 | 2 |
| Yb4 Sb4 Pd4 | mp-20540 | 2 |
| V8 P4 | mp-20541 | 0 |
| Y4 Si4 Ni4 | mp-20557 | 2 |
| Ni12 B4 | mp-2058 | 2 |
| Tb4 Si4 Ru4 | mp-20645 | 0 |
| Ca8 In4 | mp-20669 | 0 |
| U4 Co4 Ge4 | mp-20671 | 3 |
| Zr4 Ni4 Sb4 | mp-20697 | 0 |

| | | |
|---|---|---|
| Cr4 As4 | mp-20717 | 1 |
| Np4 Si4 | mp-20765 | 1 |
| Er8 Re4 C8 | mp-20799 | 1 |
| U4 Co4 Si4 | mp-20811 | 0 |
| Tm4 Ge4 Ru4 | mp-20888 | 3 |
| Zr4 Fe4 P4 | mp-20892 | 3 |
| Ge4 Ir4 | mp-208 | 2 |
| Nb4 Ni4 P8 | mp-20948 | 2 |
| Y8 Re4 C8 | mp-21003 | 1 |
| Pr4 Sn4 Ru4 | mp-21010 | 3 |
| Pr4 Ge4 | mp-2102 | 0 |
| Cr4 P4 | mp-21048 | 3 |
| Ta4 Mn4 P4 | mp-21066 | 0 |
| Y4 Si4 Ru4 | mp-21069 | 0 |
| La4 Yb4 S12 | mp-21106 | 0 |
| Tm4 Ni4 Ge4 | mp-21157 | 0 |
| Sc12 P8 | mp-21182 | 2 |
| Mn28 C12 | mp-21256 | 0 |
| Ti4 Co4 Si4 | mp-21306 | 0 |
| Tb4 Ge4 Ru4 | mp-21310 | 0 |
| La4 Ge4 | mp-21345 | 0 |
| Sb4 Rh8 | mp-21359 | 0 |
| Tb4 Sn4 Pd4 | mp-21401 | 0 |
| Tb4 Ni4 Ge4 | mp-21424 | 2 |
| Yb4 Mn4 Si4 | mp-21439 | 2 |
| Nb4 Co4 P4 | mp-21449 | 3 |
| Pr4 Sn4 Pt4 | mp-21453 | 1 |
| Co4 Re4 B4 | mp-21464 | 2 |
| B4 Rh8 | mp-21502 | 3 |
| La4 In16 Au8 | mp-21523 | 0 |
| Sr12 Ni12 N12 | mp-21524 | 2 |
| Ba4 Sm8 Cu4 O20 | mp-21568 | 1 |
| Y24 Te8 Rh4 | mp-21621 | 3 |
| Ba12 Ni12 N12 | mp-21653 | 2 |
| Y4 Si12 Ni20 | mp-21661 | 2 |
| Nb20 Ge16 | mp-21681 | 2 |
| La20 Pb16 | mp-21691 | 0 |
| Ca12 Ge12 Au12 | mp-21710 | 2 |
| Sc8 V12 Ge16 | mp-21719 | 0 |
| Ba20 Al4 Ir8 O44 | mp-21742 | 1 |
| Ca12 Cu12 Ge12 | mp-21779 | 2 |
| Y4 Ni20 Ge12 | mp-21806 | 0 |
| U8 Nb12 Ge16 | mp-21813 | 1 |
| P4 Ru8 | mp-21911 | 0 |
| Y12 Ni12 Sn24 | mp-21981 | 0 |
| La4 Ti4 O12 | mp-22013 | 0 |
| Ti20 Sb12 | mp-22033 | 3 |
| Zr4 Sb4 Pd4 | mp-22036 | 0 |
| Ho4 Ge4 Ru4 | mp-22041 | 3 |
| Lu4 Ge4 Ru4 | mp-22051 | 3 |
| Yb4 F12 | mp-22072 | 0 |
| Tb4 Sb4 Rh4 | mp-22115 | 1 |
| Pr4 Ni4 Sn4 | mp-22164 | 2 |
| Zr12 Ni4 Sb28 | mp-22174 | 1 |
| Co8 P4 | mp-22204 | 3 |
| Zr4 Mn4 Si4 | mp-22227 | 3 |
| Tb4 Sn4 Pt4 | mp-22238 | 1 |
| Ge4 Rh4 | mp-22239 | 2 |

| | | |
|---|---|---|
| Zr4 P4 Ru4 | mp-22268 | 0 |
| Y4 Sn4 Pt4 | mp-22275 | 1 |
| Sr4 In4 Pt4 | mp-22284 | 2 |
| Tb4 Ni4 Sn4 | mp-22299 | 2 |
| Tb4 Ge4 Pt4 | mp-22324 | 1 |
| Sc4 Si4 Ni4 | mp-22426 | 0 |
| Hf4 Fe4 P4 | mp-22434 | 3 |
| Mo4 P4 Ru4 | mp-22451 | 2 |
| Hf4 Cu4 Si4 | mp-22489 | 0 |
| Ho4 Si4 Ru4 | mp-22497 | 3 |
| Zr4 Cu4 Si4 | mp-22522 | 0 |
| Co4 As4 Rh4 | mp-22546 | 3 |
| Ba4 Dy8 Cu4 O20 | mp-22550 | 1 |
| Pr8 Re4 C8 | mp-22561 | 1 |
| Sc12 As8 | mp-22575 | 1 |
| Sc12 P8 | mp-22600 | 2 |
| Y4 Ni4 Sn4 | mp-22617 | 2 |
| Ta4 Ni4 Ge4 | mp-22636 | 3 |
| Pr4 Sn4 Pd4 | mp-22645 | 0 |
| In4 Pd8 | mp-22646 | 0 |
| Ba4 Pr4 O12 | mp-22705 | 0 |
| Ta4 Ni4 B8 | mp-22709 | 0 |
| Nb4 Si4 Pd4 | mp-22722 | 1 |
| Ni4 Bi12 | mp-23179 | 2 |
| Li4 B4 H4 | mp-23694 | 2 |
| P4 W4 | mp-2420 | 2 |
| Pr8 Au4 | mp-2714 | 2 |
| Nb8 P20 | mp-27672 | 3 |
| Y4 Si4 Pd8 | mp-28024 | 0 |
| Al4 Pd8 | mp-2824 | 2 |
| Nb4 Te20 Pd4 | mp-28616 | 1 |
| Ta4 Ni8 Te8 | mp-28667 | 1 |
| Nb12 Ge4 Te24 | mp-28754 | 0 |
| Y8 Al4 Ge12 | mp-28997 | 2 |
| Lu4 B8 Ru4 | mp-29239 | 1 |
| Na4 Ti8 O16 | mp-29356 | 2 |
| Ca20 Sn20 Au20 | mp-29561 | 3 |
| Sc20 Ni8 Te8 | mp-29769 | 0 |
| Hf12 P12 Pd16 | mp-29811 | 3 |
| Sc24 Ag4 Te8 | mp-30203 | 2 |
| Ba12 P12 I8 | mp-30220 | 1 |
| Ca12 Au4 | mp-30366 | 2 |
| Ho8 Au4 | mp-30385 | 2 |
| Sc12 Mn8 Ga24 | mp-30652 | 3 |
| Pr4 Cu24 | mp-30698 | 3 |
| Sc12 Ga24 Fe8 | mp-30701 | 2 |
| Ho4 Zn12 | mp-30736 | 3 |
| La20 Sn16 | mp-30757 | 0 |
| La4 Sn4 Pt4 | mp-3076 | 2 |
| Y4 Zn12 | mp-30884 | 1 |
| Ca4 Ga4 Pt4 | mp-31152 | 2 |
| Ho4 Ni4 Sn4 | mp-31176 | 2 |
| Sr12 Sn12 Au12 | mp-31281 | 2 |
| La12 Sn24 Pd16 | mp-31295 | 0 |
| Ca12 Ga12 Ir8 | mp-31481 | 1 |
| Fe4 As4 | mp-427 | 2 |
| Mg4 Al4 Si4 | mp-4499 | 2 |
| Ag4 As4 F28 | mp-4807 | 3 |

| | | |
|---|---|---|
| Ca4 Nb4 O12 | mp-4957 | 0 |
| Nb4 Ni4 As8 | mp-504835 | 2 |
| Ni8 Sn4 P4 | mp-504909 | 3 |
| Ti8 Ni4 P20 | mp-505081 | 2 |
| Nb12 Si4 Te24 | mp-505137 | 0 |
| Ta12 Si4 Te24 | mp-505206 | 0 |
| Ba4 Lu8 Cu4 O20 | mp-505268 | 1 |
| Ce4 Ge4 Rh4 | mp-505282 | 1 |
| Ba8 Re4 O20 | mp-505390 | 2 |
| Na12 Fe8 Se16 | mp-505443 | 0 |
| Ce8 Sc12 Si16 | mp-505512 | 0 |
| Cr20 As12 | mp-505539 | 0 |
| Zr20 Sb12 | mp-505759 | 1 |
| Sc4 Ni4 Sn4 | mp-5186 | 2 |
| Zr8 Nb12 Ge16 | mp-540755 | 2 |
| Si16 Rh12 | mp-540791 | 2 |
| Tl12 Fe8 S16 | mp-541140 | 0 |
| Ca4 Yb4 In4 Se16 | mp-541276 | 2 |
| Ca4 Yb4 In4 S16 | mp-541277 | 2 |
| Zr8 Ni12 P12 | mp-541909 | 3 |
| Zr12 P12 Pd16 | mp-541951 | 3 |
| Ho4 Ni4 Ge4 | mp-542171 | 2 |
| Sc12 Si16 Ni8 | mp-542486 | 1 |
| Na4 Rh8 O16 | mp-542675 | 2 |
| Ba4 Y8 Cu4 O20 | mp-542733 | 1 |
| Ho20 Si16 | mp-542829 | 0 |
| V4 Cu4 Ag4 O16 | mp-542969 | 2 |
| Cu4 Se4 O16 | mp-554040 | 2 |
| Ca4 Ir4 O12 | mp-555735 | 2 |
| Na4 Nb4 O8 F4 | mp-557590 | 0 |
| Cs4 Al4 Ag4 F24 | mp-561999 | 3 |
| Yb20 Bi12 | mp-567280 | 3 |
| Sm8 Al4 Ge12 | mp-568449 | 0 |
| Yb4 Ag4 | mp-568629 | 1 |
| Yb4 Ge4 Ir4 | mp-568672 | 2 |
| Tm4 Al4 Rh4 | mp-568685 | 2 |
| Sr20 Ag20 | mp-568716 | 1 |
| Pr8 Sc12 Si16 | mp-568831 | 0 |
| Mg8 Co48 As28 | mp-569003 | 2 |
| Te8 Ir4 | mp-569322 | 0 |
| Yb4 Al4 Pd4 | mp-569338 | 2 |
| Lu24 Ag4 Te8 | mp-569414 | 2 |
| Al4 Au8 | mp-569558 | 2 |
| Yb8 Tl4 | mp-569605 | 1 |
| Ca4 Cd4 Au4 | mp-569628 | 2 |
| Ca20 Ir4 | mp-570356 | 3 |
| Ca4 In4 Pt4 | mp-570689 | 2 |
| Yb12 Ge12 Au12 | mp-570711 | 2 |
| Ba4 Au4 | mp-570775 | 3 |
| Yb8 Au4 | mp-570901 | 1 |
| Hf16 Nb4 Ge16 | mp-571038 | 2 |
| Tb8 Al4 Ge12 | mp-571381 | 0 |
| Yb8 In4 | mp-581760 | 0 |
| Ca20 Cu20 | mp-585949 | 1 |
| Ce4 Ga4 Ni4 | mp-600663 | 2 |
| Al4 Pd20 | mp-605663 | 0 |
| Ca12 Ga12 Rh8 | mp-607230 | 3 |
| Pr4 In16 Au8 | mp-607514 | 0 |

| | | |
|---|---|---|
| Ca4 In4 Pd4 | mp-620571 | 2 |
| P12 Rh16 | mp-621581 | 3 |
| Ta4 Ni8 Te4 Se4 | mp-622009 | 0 |
| Al12 Ni4 | mp-622209 | 2 |
| Pr8 Ga4 | mp-623027 | 0 |
| Pr4 Ga4 Co4 | mp-623261 | 0 |
| Tb12 Ni4 | mp-623751 | 0 |
| Cu28 S16 | mp-624299 | 2 |
| Ca8 In16 Au12 | mp-630875 | 1 |
| La4 Cu24 | mp-636256 | 3 |
| Ni16 B12 | mp-640067 | 2 |
| Ho20 Ni4 Sb8 | mp-640383 | 1 |
| Y24 Ag4 Te8 | mp-642238 | 2 |
| Y28 Te8 | mp-642301 | 2 |
| Lu24 Cu4 Te8 | mp-642315 | 2 |
| Pr12 Ge24 Pt16 | mp-645543 | 3 |
| Li4 Yb16 Ge16 | mp-646071 | 1 |
| Zr4 Rh4 | mp-669917 | 1 |
| Y20 Pb16 | mp-672188 | 1 |
| Tb12 Ni12 | mp-672240 | 0 |
| Ce4 Al20 Pt12 | mp-672344 | 1 |
| Ti4 Si4 Rh4 | mp-672645 | 3 |
| Hf8 Nb12 Ge16 | mp-672696 | 2 |
| Yb28 Cl60 | mp-680254 | 0 |
| Ti20 P12 | mp-680570 | 0 |
| La12 Yb12 S36 | mp-684002 | 2 |
| Sc4 Ni4 Ge4 | mp-7066 | 0 |
| Tb4 Si4 Pt4 | mp-7124 | 3 |
| Y12 Pt4 | mp-7343 | 0 |
| Sb4 Ru4 | mp-7565 | 2 |
| Lu12 Ni12 Sn24 | mp-7736 | 1 |
| U4 V4 C8 | mp-7810 | 1 |
| Ti4 B4 | mp-7857 | 0 |
| Si4 Rh4 | mp-818 | 2 |
| Ca4 Sb4 Pt4 | mp-8487 | 2 |
| Yb8 Al4 Ge12 | mp-864676 | 1 |
| Yb4 Ga4 Pt4 | mp-864912 | 2 |
| Sc4 Si4 Pt4 | mp-9225 | 2 |
| Tb8 Re4 C8 | mp-972246 | 1 |
| Lu4 Ni4 Sn4 | mp-977588 | 2 |
| Y8 Au4 | mp-979911 | 2 |
| Pr4 Si4 | mp-9968 | 0 |
| Mo4 As4 | mp-9998 | 2 |
